# Supplementary material for: Magnon gap excitations and spin-entangled optical transition in van der Waals antiferromagnet NiPS3
Source: arXiv:2306.07660 source file (2023-06-13)
Supplement: Supplementary file 1 [file NiPS3_Magnon_SM_Dipankar.pdf]

# Supplemental Material for "Magnon excitations and spin-entangled excitons in van der Waals antiferromagnet $NiPS_3$"

Dipankar Jana,[1,*] P. Kapuscinski,[1] I. Mohelsky,[1] D. Vaclavkova,[1] I. Breslavetz,[1] M. Orlita,[1,2] C. Faugeras,[1] and M. Potemski[1,3,†]

[1] *Laboratiore National des Champs Magnétiques Intenses, LNCMI-EMFL, CNRS UPR3228, Univ. Grenoble Alpes, Univ. Toulouse, Univ. Toulouse 3, INSA-T, Grenoble and Toulouse, France*

[2] *Institute of Physics, Charles University, Ke Karlovu 5, Prague, 121 16, Czech Republic*

[3] *CENTERA Labs, Institute of High Pressure Physics, PAS, 01 - 142 Warsaw, Poland*

## I. EXPERIMENTAL DETAILS

### A. Sample preparation

As already mentioned in the main text, the samples used in our experiments were extracted from commercially available bulk $NiPS_3$ crystals. The crystals we have used were not however perfectly homogeneous but composed of "twisted" grains, with different crystal axis orientations in the layers', a-b plane. The isolation of single crystals (with well defined, a,b crystallographic axes in their entire volume), has been a critical point for the majority of the experiments presented in our work. These experiments (micro-Raman and micro-photoluminescence measurements versus in-plane magnetic field $B$) has been carried out on relatively small size flakes exfoliated from bulk $NiPS_3$ crystals and transferred on silicon substrates. Each flake has been primarily characterized by polarization resolved photoluminescence (PL) measurements (at low temperature and $B = 0$) of the X-transition (see the main text). The X-transition is linearly polarized because it is coupled to spins which are aligned along the a-crystal axis [S1]. In the ideal case of perfectly uniform $NiPS_3$ crystals, the polarization degree of the X-emission is expected to reach the unity. The compromise criterion to select samples for further experiments was to choose those which display the polarization degree larger than 0.8. The issue of the crystal homogeneity was not however essential for the experiments carried out as a function of the magnetic field applied perpendicularly to the layer planes. In such a geometry, the direction of the spin alignment is always perpendicular to the applied magnetic field, independent on the crystallites' orientation in the a,b plane. Thus, using large samples unavoidable for far-infrared transmission measurements was justified in experiments with Faraday-geometry.

### B. Experimental set-up

Micro-optical arrangement has been applied in all Raman scattering and photoluminescence measurements presented in our work. The continuous-wave laser operational at 515 nm was used as the excitation source. The laser beam has been focused via 50 X microscope objectives providing $\sim 2\ \mu m$ in diameters spot on the samples. The emitted/scattered light, collected via the same objective, was dispersed with a 0.7 m long monochromator and detected with a nitrogen-cooled charge coupled device camera. Experiments as a function of temperature are carried out by placing sample on the cold finger of a continuous flow cryostat which is mounted on x-y positioners. In case of measurements conducted as a function of the magnetic field we used a free-beam insert placed in a superconducting magnet supplying the magnetic fields up to 14 T. The x-y-z piezo stage with the sample placed on it and microscope objective fixed above have been altogether immersed in a tube filled in with gaseous helium, in contacts with bath of liquid helium.

When measuring the Raman scattering signals, special efforts have been made to efficiently reject the stray laser light. First of all, both the excitation beam and the out-coming light were passed through the sets of triple Bragg filters. To further suppress the stray laser light a certain angle was set between the direction of the incident laser beam and the direction normal to the surface sample (crystal c-axis). This angle was fixed at 20° in case of field dependent experiments, the results of which are presented in Fig. 3, Fig. 5 and Fig. 8 of main text. It was fixed at 30° in the experiments carried out as a function of temperature (see Fig. 2 of the main text and Fig. S1). It should be,

* dipankar.jana@lncmi.cnrs.fr
† marek.potemski@lncmi.cnrs.fr

however, noted that the direction of the excitation beam was kept parallel to the c-axis in case of photoluminescence measurements illustrated in Fig. 7 of the main text.

Far-infrared magneto-transmission experiments were carried out on large area $NiPS_3$ specimens which were kept in helium exchange gas at temperature of 4.2 K and placed in a superconducting solenoid magnet. The magnetic field was always applied perpendicular to the quasi-two-dimensional plane and aligned with the wave vector of the probing radiation (Faraday configuration). To measure the magneto-transmission, the radiation from a mercury lamp was modulated by a Bruker Vertex 80v Fourier-transform spectrometer, delivered to the sample via light-pipe optics and then detected by a composite bolometer placed directly behind the sample.

## II. RAMAN SCATTERING RESPONSE OF NIPS$_3$ IN A WIDE SPECTRAL RANGE: MAGNON AND PHONON EXCITATIONS

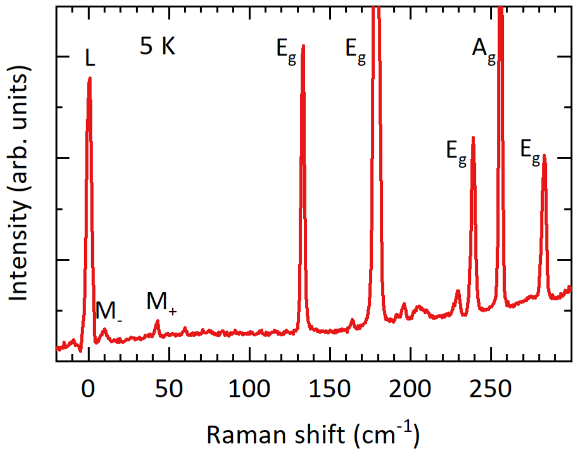


FIG. S1. Low temperature (10 K) Raman scattering spectrum of $NiPS_3$ in a broad energy range. $M_-$ and $M_+$ peaks are due to magnon gap excitations extensively characterized in the main text, whereas $E_g$ and $A_g$ denote the symmetries of the characteristic phonon excitations identified in previous studies [S2–S4].

Our Raman scattering study presented in the main text, has been focused on the low energy excitations which appear in the close vicinity of the laser line. We have, however, also measured the Raman scattering spectra in a wide spectral range. An example of such a spectrum is illustrated in Fig. S1. The features seen in this spectrum at energies above 50 $cm^{-1}$ are due to characteristic phonon excitations in $NiPS_3$, that has been previously reported and characterized [S2–S4]. We note that Raman peaks due to phonon excitations are significantly more intense that those associated to $M_+$ and $M_-$ magnon gap excitations which are the central point of the present work.

## III. NUMERICAL SIMULATIONS FOR THE IN-PLANE MAGNETIC FIELD DEPENDENT SPIN ROTATION AND MAGNON GAP ENERGIES

As discussed in the main part of the text, the evolution, upon the application of the in-plane magnetic field, of magnon gaps and the associated rotation of the spin ensemble in $NiPS_3$ antiferromagnet can be described with the solutions of Eq. 1 and Eq. 3 of the main text. Critical parameter in these solutions is the angle $\theta_B$ between the direction of the applied field and the magnetic moment alignment (i.e. the crystal a-axis) in the absence of the magnetic field. A pictorial illustration of the rotation of the spin assembly in $NiPS_3$ upon application of the in-plane magnetic field aligned at certain $\theta_B \neq 0$ angle is presented in Fig. S2. When increasing the magnetic field, the spins rotate towards the direction perpendicular to the magnetic field, the rotation being quantified by the angle $\Psi$ between the field direction and the apparent axis of the spin alignment. At sufficiently high fields, above the spin flop field, the spins are aligned nearly perpendicular to the magnetic field ($\Psi \sim 90°$). Obviously, upon further increase of the magnetic field the antiferromagnetic spin order should progressively turn into the ferromagnetic one with all spins aligned along the field direction. The numerical solution of the Eq. 1 and Eq. 3, for the B-dependence of $\Psi$ , $w_{M-}$ and $w_{M+}$ are presented in Fig. S3 for several selected angle $\theta_B$. All traces in these figures have been plotted

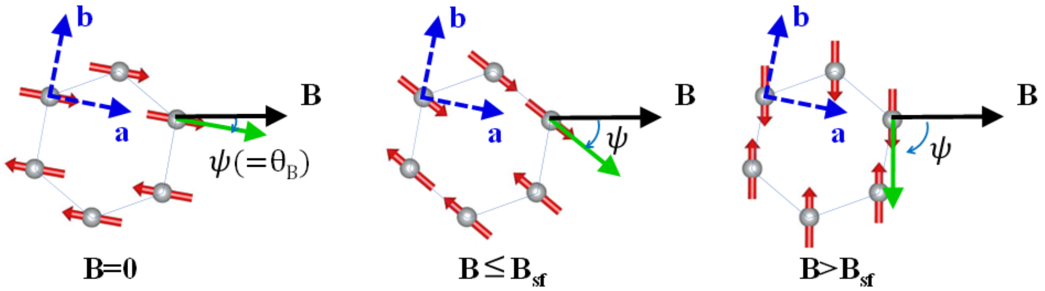


FIG. S2. A pictorial illustration of the rotation of the spin assembly in $NiPS_3$ upon application of the in-plane magnetic field.

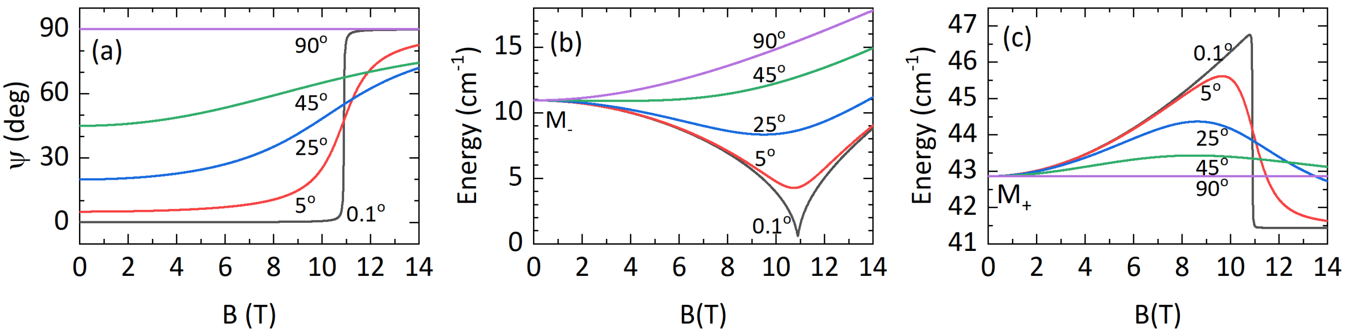


FIG. S3. (a) Simulated in-plane magnetic field dependence of $\Psi$ for different values of $\theta_B$, (b) and (c) Simulated in-plane magnetic field dependence of low $M_-$ and high $M_+$ energy magnon modes respectively for different $\theta_B$.

assuming a common set of other parameters: $g = 2.15$, $w_{M-} = 11\ cm^{-1}$ and $w_{M+} = 42.7\ cm^{-1}$ respectively, for the g-factor and two magnon gap energies at $B = 0$T (see the main text). The results of calculations shown in Fig.S3 are in support to the analysis of the experimental data presented in Fig. 4 of the main text. To this end it is worth noting that analytical solutions can be obtained in the limit of $\theta_B = 0°$. As already presented in the main text, $w_{M+} = g\mu_B\sqrt{C_2 + 3B^2}$ and $w_{M-} = g\mu_B\sqrt{C_1 - B^2}$ for $B \leq B_{sf}$. When $B \geq B_{sf}$, the field dependence of magnon mode energies are given by [S5] $w_{M-} = g\mu_B\sqrt{B^2 - C_1}$ and $w_{M+} = g\mu_B\sqrt{C_2 - C_1}$. Spins remain aligned along the a-axis until the spin-flop field at which they rotate abruptly to align perpendicularly to the magnetic field (along the b-crystal axis).

## IV. IN-PLANE MAGNETIC FIELD DEPENDENT ROTATION OF X-TRANSITION PL POLARIZATION

As mentioned before, the X-transition is expected to be linearly polarized due to coupling with spin alignment. The rotation of the $Ni^{2+}$ spins' alignment induced by the application of the in-plane magnetic field (see Fig. S3 (a)) will therefore impose the rotation of the axis of linear polarization of X-transition. This effect is illustrated in Fig. S4, for the case when the applied magnetic field is nearly parallel ($\theta_B = 5°$) to the initial (at $B = 0$ T) alignment of $Ni^{2+}$ spins (the data are complementary to those presented in Fig. 7 of the main text). A high degree of linear polarization confirms unidirectional spin orientation of the investigated flake while the significant turn of the PL polarization axis after the spin-flop field establishes the field-induced spin rotation.

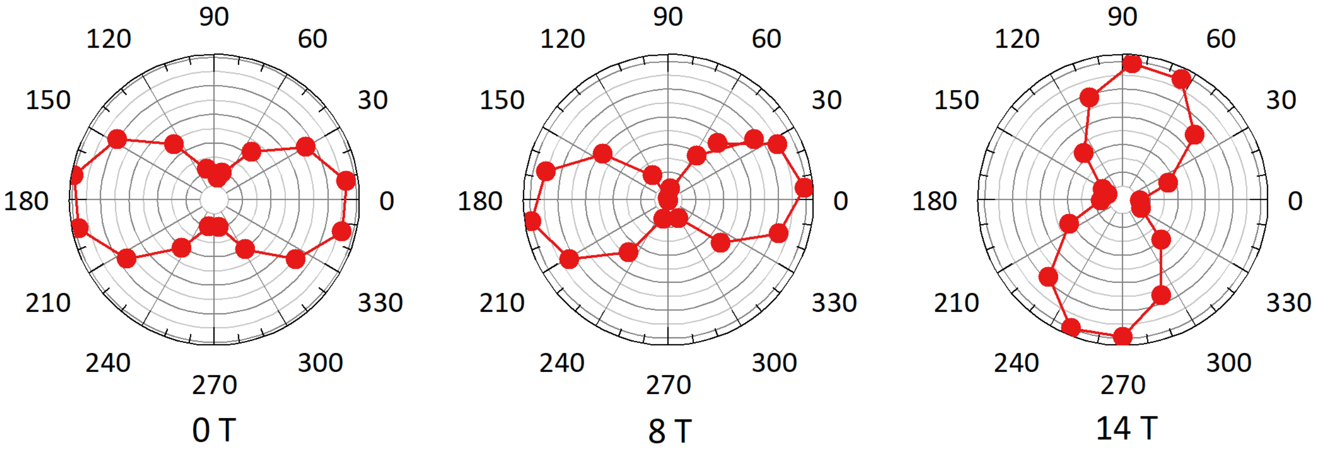


FIG. S4. Polar plots of linear polarization resolved integrated photoluminescence intensity of the upper component of the $X_+$-transition at different magnetic fields applied in the in-plane direction (the corresponding traces for the $X_-$-component are identical). The presented data complete those presented in Fig. 7 of the main text. Both data sets have been obtained for the same $NiPS_3$ flake, and the geometry of the applied field was also the same. A contribution of Faraday rotation induced by the objective lens has been subtracted and the polarization orientation at $B = 0$ T was a taken as a reference and set as $0^{\circ\circ}$ axis.

[S1] Q. H. Wang, A. Bedoya-Pinto, M. Blei, A. H. Dismukes, A. Hamo, S. Jenkins, M. Koperski, Y. Liu, Q.-C. Sun, E. J. Telford, *et al.*, The magnetic genome of two-dimensional van der waals materials, ACS nano **16**, 6960 (2022).

[S2] X. Wang, J. Cao, Z. Lu, A. Cohen, H. Kitadai, T. Li, Q. Tan, M. Wilson, C. H. Lui, D. Smirnov, *et al.*, Spin-induced linear polarization of photoluminescence in antiferromagnetic van der waals crystals, Nature Materials **20**, 964 (2021).

[S3] S. Y. Kim, T. Y. Kim, L. J. Sandilands, S. Sinn, M.-C. Lee, J. Son, S. Lee, K.-Y. Choi, W. Kim, B.-G. Park, *et al.*, Charge-spin correlation in van der waals antiferromagnet $NiPS_3$, Physical review letters **120**, 136402 (2018).

[S4] C. Kim, J. Jeong, P. Park, T. Masuda, S. Asai, S. Itoh, H.-S. Kim, A. Wildes, and J.-G. Park, Spin waves in the two-dimensional honeycomb lattice xxz-type van der waals antiferromagnet cops 3, Physical Review B **102**, 184429 (2020).

[S5] S. M. Rezende, A. Azevedo, and R. L. Rodríguez-Suárez, Introduction to antiferromagnetic magnons, Journal of Applied Physics **126**, 151101 (2019).
